# Supplementary material for: Online Continual Learning with Maximally Interfered Retrieval
Source: arXiv:1908.04742 source file (2019-10-29)
Supplement: Supplementary file 1 [file Donot_submit.tex]

\documentclass{article}

% if you need to pass options to natbib, use, e.g.:
%     \PassOptionsToPackage{numbers, compress}{natbib}
% before loading neurips_2019

% ready for submission
% \usepackage{neurips_2019}

% to compile a preprint version, e.g., for submission to arXiv, add add the
% [preprint] option:
%     \usepackage[preprint]{neurips_2019}

% to compile a camera-ready version, add the [final] option, e.g.:
\usepackage[]{neurips_2019}
\usepackage{bm}
% to avoid loading the natbib package, add option nonatbib:
%     \usepackage[nonatbib]{neurips_2019}
\usepackage[utf8]{inputenc} % allow utf-8 input
\usepackage{amsmath,amsfonts}
\usepackage[algo2e,ruled,linesnumbered,lined]{algorithm2e}
\usepackage[T1]{fontenc}    % use 8-bit T1 fonts
\usepackage[draft]{hyperref}       % hyperlinks
\usepackage{url}            % simple URL typesetting
\usepackage{booktabs}       % professional-quality tables
\usepackage{amsfonts}       % blackboard math symbols
\usepackage{nicefrac}       % compact symbols for 1/2, etc.
\usepackage{microtype}      % microtypography
\usepackage{color}
\usepackage{graphicx}
\usepackage{tabu}
\usepackage{caption}
\usepackage{subcaption}
\usepackage{wrapfig,lipsum,booktabs}

\title{This is not Supplementary file}

% The \author macro works with any number of authors. There are two commands
% used to separate the names and addresses of multiple authors: \And and \AND.
%
% Using \And between authors leaves it to LaTeX to determine where to break the
% lines. Using \AND forces a line break at that point. So, if LaTeX puts 3 of 4
% authors names on the first line, and the last on the second line, try using
% \AND instead of \And before the third author name.

\author{%
  David S.~Hippocampus\thanks{Use footnote for providing further information
    about author (webpage, alternative address)---\emph{not} for acknowledging
    funding agencies.} \\
  Department of Computer Science\\
  Cranberry-Lemon University\\
  Pittsburgh, PA 15213 \\
  \texttt{hippo@cs.cranberry-lemon.edu} \\
  % examples of more authors
  % \And
  % Coauthor \\
  % Affiliation \\
  % Address \\
  % \texttt{email} \\
  % \AND
  % Coauthor \\
  % Affiliation \\
  % Address \\
  % \texttt{email} \\
  % \And
  % Coauthor \\
  % Affiliation \\
  % Address \\
  % \texttt{email} \\
  % \And
  % Coauthor \\
  % Affiliation \\
  % Address \\
  % \texttt{email} \\
}

\begin{document}

\maketitle

\section{Interference guided sampling} 
Assume that the function $p^\theta(y|x)$ parameterized by $\theta$ is the classifier we want to learn. In order to prevent catastrophic forgetting for the classifier, we also introduce a generative model $p^\gamma(x)$ which captures the input distribution of the previously observed $x$. During training of classifier on the data pair $(x_t, y_t)$, the update on the classifier parameter $\theta$ could cause catastrophic interference for the previous pairs $(x_i, y_i);\forall{i}\in{[0..t-1]}$. In order to prevent forgetting, a naive way would be to resample the previous observations from $p(x, y)=p^\gamma(x)p^\theta(y|x)$ before the update. 

To be more efficient than the naive method, we suggest to retrieve samples that would be (maximally) interfered by learning on the new data. This is motivated by the idea that the loss of many previous data samples could be unaffected or even improved, thus retraining on all of them is wasteful.

To compute the interference introduced by updating on $(x_t, y_t)$, we perform a virtual update on $\theta$: $\theta^v=\theta-\alpha\nabla_\theta\mathcal{L}(p^\theta(y|x_t),y_t)$ where $\mathcal{L}(p^\theta(y|x_t), y_t)$ is the classification loss on the current pair $(x_t, y_t)$. We then use the difference of loss before and after the virtual update as a measure of how much a sample is interfered. We simplify the loss as $\mathcal{L}^\theta(x,y)$, and define the loss difference as function $\delta$.

$$\delta(x)=\mathbb{E}_{y\sim{p^\theta(y|x)}}\left[\mathcal{L}^{\theta^v}(x,y)-\mathcal{L}^\theta(x,y)\right]$$
Sampling of $x$ should respect both $p^\gamma(x)$ and $\delta(x)$. Namely:

$$p_s(x)=p^\gamma(x)\frac{\exp{\delta(x)/T}}{Z}$$

In the case of a VAE, we don't have a probability density for $x$, but only a lower bound.

In the case of a bijector, we can further rewrite it into sampling from the latent space according to the prior $p(z)$, and mapping $z$ through the generator $G^\gamma(z)$.
$$p_s(z)=p(z)\det(\frac{\partial{z}}{\partial{x}})\frac{\exp{\delta(G^\gamma(z))/T}}{Z}$$

We can further convert $p(z)$ to polar coordinate $p(r)p(\boldsymbol{\phi})$ where $r$ is the radius and $\boldsymbol{\phi}$ are the angles. In this way, we can sample $r$ and then keep $r$ fixed when gradient ascending. Moving with $r$ fixed does not change the loss from the prior, so we're only ascending $$\log\det{\frac{\partial{z}}{\partial{x}}}+\delta(G^\gamma(z))/T$$

\end{document}
